# Supplementary material for: On Estimating Degree Distribution in Streaming and Query Models
Source: arXiv:2507.21784 source file (2026-10-12)
Supplement: Supplementary file 1 [file 4_Enlarged_Plots.tex]

\clearpage
\newpage

% In this section, we present the experimental results in more detail. 

\subsection{Experimental Results}

In this section, we present the numerical data for the results presented in \Cref{Section: experiment}.

\begin{table}[htbp]
\centering
\small
\begin{tabular}{rrrrrr}
\toprule
$c$ &
Error at $\frac{2h}{5}$ &
Error at $\frac{4h}{5}$ &
Error at $h$ &
Error at $\frac{2\degree{\max{}}+3h}{5}$ &
Error at $\frac{4\degree{\max{}}+h}{5}$ \\
\midrule
0.0025 & 0.08 & 0.14 & 0.18 & 0.08 & 0.05 \\
0.005  & 0.06 & 0.09 & 0.10 & 0.05 & 0.03 \\
0.01   & 0.04 & 0.07 & 0.06 & 0.03 & 0.02 \\
0.025  & 0.03 & 0.04 & 0.02 & 0.02 & 0.02 \\
0.05   & 0.02 & 0.03 & 0.01 & 0.01 & 0.01 \\
0.10   & 0.01 & 0.02 & 0.01 & 0.01 & 0.01 \\
0.25   & 0.01 & 0.01 & 0.00 & 0.00 & 0.00 \\
0.50   & 0.00 & 0.01 & 0.00 & 0.00 & 0.00 \\
\bottomrule
\end{tabular}
\caption{Estimation error at different degrees at various choices of the constant $c$ (\Cref{fig:CvsErrH})}
\label{tab:error-vs-c}
\end{table}


\begin{table}[htbp]
\centering
\small
\begin{tabular}{lrrrrrrr}
\toprule
& \multicolumn{3}{c}{Graph Parameters} & \multicolumn{4}{c}{Estimation Error} \\
\cmidrule(lr){2-4} \cmidrule(lr){5-8}
Graph &
\#Vertices &
\#Edges &
h-index &
Fraction of&
Error at  &
Error at &
Error at \\

Name &
($n$) ($\times 10^{6}$) &
($m$) ($\times 10^{6}$) &
($h$) &
Queries (\%) &
$\frac{4h}{5}$ &
$h$ &
$\frac{2\degree{\max{}}+3h}{5}$ \\
\midrule
wiki-ch-intrnl & 1.93 & 8.96 & 950 & 1.52 & 0.08 & 0.07 & 0.03 \\
hudong & 1.98 & 14.62 & 1{,}330 & 1.09 & 0.08 & 0.10 & 0.01 \\
Baidu-Baike & 2.14 & 17.03 & 1{,}227 & 1.19 & 0.07 & 0.08 & 0.01 \\
Wikipedia-DE & 3.78 & 68.85 & 2{,}286 & 0.66 & 0.06 & 0.08 & 0.01 \\
Wikipedia-IT & 2.79 & 86.81 & 2{,}400 & 0.62 & 0.09 & 0.12 & 0.00 \\
Wikipedia-FR & 4.91 & 105.63 & 3{,}107 & 0.50 & 0.11 & 0.13 & 0.00 \\
indochina-2004 & 7.41 & 153.49 & 6{,}986 & 0.23 & 0.12 & 0.03 & 0.04 \\
uk-2002 & 18.48 & 267.66 & 2{,}796 & 0.60 & 0.07 & 0.09 & 0.01 \\
\bottomrule
\end{tabular}
\caption{ Estimation error for various Web Graphs at $\constant = 0.01$ (\Cref{Fig: WebErrH,Fig: WebErrdmin2h})}
\label{tab:empirical-summary-wiki}
\end{table}


\begin{table}[htbp]
\centering
\small
\begin{tabular}{lrrrrrrr}
\toprule
& \multicolumn{3}{c}{Graph Parameters} & \multicolumn{4}{c}{Estimation Error} \\
\cmidrule(lr){2-4} \cmidrule(lr){5-8}
Graph &
\#Vertices &
\#Edges &
h-index &
Fraction of&
Error at  &
Error at &
Error at \\

Name &
($n$) ($\times 10^{6}$) &
($m$) ($\times 10^{6}$) &
($h$) &
Queries (\%) &
$\frac{4h}{5}$ &
$h$ &
$\frac{2\degree{\max{}}+3h}{5}$ \\
\midrule
flixster & 2.52 & 7.92 & 957 & 1.54 & 0.06 & 0.02 & 0.14 \\
LiveJournal & 4.03 & 27.93 & 558 & 2.73 & 0.03 & 0.04 & 0.05 \\
fb-UCI-UNI & 58.79 & 92.21 & 1{,}234 & 1.45 & 0.03 & 0.05 & 0.03 \\
fb-konnect & 59.22 & 92.52 & 1{,}234 & 1.45 & 0.03 & 0.04 & 0.03 \\
Orkut & 3.00 & 106.35 & 1{,}522 & 0.98 & 0.05 & 0.06 & 0.01 \\
lj-user-groups & 7.49 & 112.31 & 3{,}712 & 0.43 & 0.09 & 0.10 & 0.00 \\
sinaweibo & 58.66 & 261.32 & 5{,}902 & 0.30 & 0.02 & 0.06 & 0.00 \\
twitter-2010 & 21.30 & 265.03 & 6{,}189 & 0.27 & 0.07 & 0.08 & 0.00 \\
\bottomrule
\end{tabular}
\caption{Estimation error for various Social Networks at $\constant = 0.01$ (\Cref{Fig: SocErrH,Fig: SocErrdmin2h})}
\label{tab:empirical-summary}
\end{table}



\begin{table}[htbp]
\centering
\small
\begin{tabular}{llrrr}
\toprule
& & \multicolumn{3}{c}{Graph Parameters} \\
\cmidrule(lr){3-5}
Graph Type & Graph Name &
\#Vertices ($\times 10^{6}$) &
\#Edges ($\times 10^{6}$) &
h-index ($h$) \\
\midrule
Web & web-uk-2002 & 18.48 & 267.66 & 2{,}796 \\
Social Network & twitter-2010 & 21.30 & 265.03 & 6{,}189 \\
Social Network & sinaweibo & 58.66 & 261.32 & 5{,}902 \\
Web & web-indochina-2004 & 7.41 & 153.49 & 6{,}986 \\
Social Network & lj-user-groups & 7.49 & 112.31 & 3{,}712 \\
Social Network & Orkut & 3.00 & 106.35 & 1{,}522 \\
Web & Wikipedia-FR & 4.91 & 105.63 & 3{,}107 \\
Social Network & fb-konnect & 59.22 & 92.52 & 1{,}234 \\
Social Network & fb-UCI-UNI & 58.79 & 92.21 & 1{,}234 \\
Web & Wikipedia-IT & 2.79 & 86.81 & 2{,}400 \\
Web & Wikipedia-DE & 3.78 & 68.85 & 2{,}286 \\
Miscellaneous & ca-hollywood-2009 & 1.07 & 56.31 & 2{,}584 \\
Social Network & LiveJournal & 4.03 & 27.93 & 558 \\
Web & Baidu-Baike & 2.14 & 17.03 & 1{,}227 \\
Miscellaneous & cit-Patents & 3.77 & 16.52 & 237 \\
Miscellaneous & ca-coauthors-DBLP & 0.54 & 15.25 & 512 \\
Web & hudong & 1.98 & 14.62 & 1{,}330 \\
Miscellaneous & as-skitter & 1.70 & 11.10 & 982 \\
Web & wiki-ch-internal & 1.93 & 8.96 & 950 \\
Social Network & dogster & 0.43 & 8.55 & 1{,}268 \\
Social Network & flixster & 2.52 & 7.92 & 957 \\
Web & web-it-2004 & 0.51 & 7.18 & 431 \\
Social Network & myspace & 0.85 & 6.49 & 649 \\
Web & Stanford & 0.28 & 1.99 & 427 \\
Social Network & fb-UF21 & 0.04 & 1.47 & 371 \\
Miscellaneous & loc-gowalla & 0.20 & 0.95 & 275 \\
Web & BerkStan & 0.03 & 0.16 & 157 \\
Web & webbase-2001 & 0.02 & 0.03 & 65 \\
Web & web-google & 0.00 & 0.00 & 20 \\
\bottomrule
\end{tabular}
\caption{Graph parameters for various real-world graphs (\Cref{fig:NvsM,fig:HvsN})}
\label{tab:graph-statistics-sorted}
\end{table}

\subsection{Enlarged Plots}

In this section, we present enlarged versions of the plots presented in \Cref{Section: experiment} to improve readability.

\begin{figure}[ht]
    \begin{minipage}{0.46\textwidth}
        \centering
        \includegraphics[width = \linewidth]{Plots/ErratConstantC005.png}
        \caption{Error at different values of $\degree{}$ for $\constant = 0.005$}
        \label{fig:ErratConstantC2}
        %\Description[]{}
        \end{minipage}\hfill
        \begin{minipage}{0.46\textwidth}
        \centering
        \includegraphics[width = \linewidth]{Plots/CvsErrorHBase.png}
        \caption{Error at $\degree{} = \hindex$ for different values of constant $\constant$}
        \label{fig:CvsErrH2}
        %\Description[]{}
    \end{minipage}
    \centering    
\end{figure}

\begin{figure}[ht]
    \begin{minipage}{0.46\textwidth}
        \centering
        \includegraphics[width=\linewidth]{Plots/HvsN.png}
        \caption{$\vertexcount$ vs $\hindex$}
        \label{fig:HvsN2}
        %\Description[]{}
        \end{minipage}\hfill
        \begin{minipage}{0.46\textwidth}
        \centering
        \includegraphics[width=\linewidth]{Plots/NvsM.png}
        \caption{$\vertexcount$ vs $\edgecount$}
        \label{fig:NvsM2}
        %\Description[]{}
    \end{minipage}
    \centering    
\end{figure}

\clearpage
\newpage


\begin{figure}[ht]
    \begin{minipage}{0.46\textwidth}
        \centering
            %\Description[]{}
            \includegraphics[ width=\linewidth]{Plots/WebErr2dminh.png}%\vspace*{-.5em}
            \caption{\small{Performance on Web graphs at $\degree{} = \nicefrac{\fbrac{2\degree{\max{}}+3\hindex}}{5}$}}\label{Fig: WebErrdmin2h2}
        \end{minipage}\hfill
        \begin{minipage}{0.46\textwidth}
        \centering
            \includegraphics[width=\linewidth]
            {Plots/WebErr4H5.png}%\vspace*{-.5em}
            \caption{\small{Performance on Web graphs at $\degree{} = \nicefrac{4\hindex}{5}$}}\label{Fig: WebErrH2}
            %\Description[]{}
    \end{minipage}
    \centering    
\end{figure}

\begin{figure}[ht]
    \begin{minipage}{0.46\textwidth}
        \centering
            \includegraphics[width=\linewidth]{Plots/SocErr2dminh.png}%\vspace*{-.5em}
            \caption{\small{Performance on SocNet graphs at $\degree{} = \nicefrac{\fbrac{2\degree{\max{}}+3\hindex}}{5}$}}\label{Fig: SocErrdmin2h2}
            %\Description[]{}     
        \end{minipage}\hfill
        \begin{minipage}{0.46\textwidth}
        \centering
            \includegraphics[width=\linewidth]{Plots/SocErr4H5.png}%\vspace*{-.5em}
            \caption{\small{Performance on Social Network graphs at $\degree{} = \nicefrac{4\hindex}{5}$}}\label{Fig: SocErrH2}
            %\Description[]{}
        \end{minipage}
    \centering    
\end{figure}
