# Supplementary material for: On Estimating Degree Distribution in Streaming and Query Models
Source: arXiv:2507.21784 source file (2026-10-12)
Supplement: Supplementary file 2 [file Ineqs.tex]

% \begin{lemma}[Median-of-Means]\label{Lem: Median-of-Means}
%     Consider a random variable $\widehat{\theta}$ is an unbiased estimator of $\theta$ with bounded mean and variance that canx be computed using $\bigo{s}$ space. Then, we can obtain an $(\approxerror,\confidence)$-estimate of $\theta$ using $\bigo{\max\sbrac{s,1},\max\sbrac{\frac{\Var(\widehat{\theta})}{\E^2[\widehat{\theta}]}\frac{1}{\approxerror^2}\log\fbrac{\frac{1}{\confidence}},1}}$ space.
% \end{lemma}
